# Supplementary material for: Effective Models for Dark Matter at the International Linear Collider
Source: arXiv:1308.4409 source file (2013-08-20)
Supplement: Supplementary file 1 [file thesis_appendix.tex]

%------------------------------------------------------------------------------
\chapter{Useful information}
\label{sec:app}
%------------------------------------------------------------------------------

In the appendix you usually include extra information that should be
documented in your thesis, but not interrupt the flow.

%%% Local Variables: 
%%% mode: latex
%%% TeX-master: "../mythesis"
%%% End: 
